# Supplementary material for: Learning Graph Structures and Uncertainty for Accurate and Calibrated Time-series Forecasting
Source: arXiv:2407.02641 source file (2024-07-02)
Supplement: Supplementary file 1 [file appendix.tex]

\appendix

\iffalse
    \section{Robustness results for \covid and \power}
    \begin{figure}[h]
        \centering
        \begin{subfigure}[b]{0.45\linewidth}
            \centering
            \includegraphics[width=.9\linewidth]{Images/noise_Covid-19.pdf}
            \caption{\covid}
        \end{subfigure}%
        \begin{subfigure}[b]{0.45\linewidth}
            \centering
            \includegraphics[width=.9\linewidth]{Images/noise_Electricity.pdf}
            \caption{\power}
        \end{subfigure}%
        \caption{\% increase in CRPS with an increase in gaussian Noise ($\rho$) added to the input sequence. Performance decrease of \model significantly lower than most of the baselines.}
        \label{fig:noise_app1}
    \end{figure}
    \begin{figure}[h]
        \centering
        \begin{subfigure}[b]{0.45\linewidth}
            \centering
            \includegraphics[width=.9\linewidth]{Images/noise_abl_Covid-19.pdf}
            \caption{\covid}
        \end{subfigure}%
        \begin{subfigure}[b]{0.45\linewidth}
            \centering
            \includegraphics[width=.9\linewidth]{Images/noise_abl_Electricity.pdf}
            \caption{\power}
        \end{subfigure}%
        \caption{\% increase in CRPS with an increase in gaussian Noise ($\rho$) added to the input sequence. Performance decrease of \model significantly lower than ablation variants.}
        \label{fig:noise_app2}
    \end{figure}
\fi
%\hk{Add Proof of ELBO}
%\hk{Add correlation tables}
